# Supplementary material for: Emergence of Interlayer Coherence in Twist-Controlled Graphene Double Layers
Source: arXiv:2206.11799 source file (2022-11-21)
Supplement: Supplementary file 1 [file SM.pdf]

# Supplemental Material for Emergence of Interlayer Coherence in Twist-Controlled Graphene Double Layers

Kenneth A. Lin, Nitin Prasad, G. William Burg, Bo Zou, Keiji Ueno, Kenji Watanabe, Takashi Taniguchi, Allan H. MacDonald, and Emanuel Tutuc

## I. Quasiparticle state energy broadening

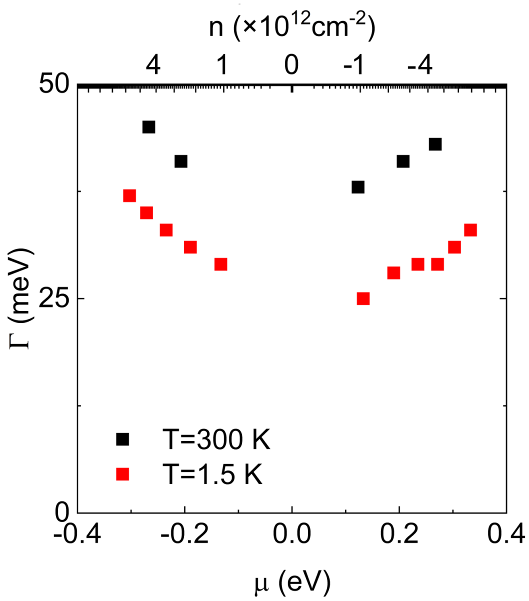


FIG. S1. Quasiparticle state energy broadening ($\Gamma$) for resonances at $V_{\text{Int}} = 0$ V under no applied magnetic field, as a function of energy $\mu$ referenced to the Dirac point of the graphene layers (bottom axis) and concentration (top axis). A fit of Eqs. 1–3 in the main text to experimental data yields $\Gamma$.

## II. Interlayer tunneling in the presence of a twist between the two layers crystal axes

When a small twist angle between the graphene layers is present, the K points of the two layers are shifted relative to each other by an amount proportional to the twist angle $\Delta\mathbf{K} = \hat{z} \times \theta\mathbf{K}$; this in turn introduces a momentum shift $\hbar\Delta\mathbf{K}$ to the tunneling carriers [1]. The momentum shift introduced by the twist angle is similar to applying an in-plane magnetic field [2]. Even a small twist angle between the top and bottom graphene layers is expected to alter tunneling characteristics significantly [3]. At $B = 0$ T with no perpendicular magnetic field applied, the momentum shift is expected to first broaden and then split the single primary resonant tunneling conductance peak into two resonance peaks, because the momentum difference is compensated by energetically shifting the two graphene layers Dirac cones by an amount $\hbar v_F \Delta\mathbf{K}$ [1], where $v_F$ is the Fermi velocity.

To assess the relative twist between the layer crystal axes in our sample, we compare the measured $g_{\mathrm{Int}}$ vs. $V_{\mathrm{Int}}$ and $V_{\mathrm{BG}}$ at a fixed $V_{\mathrm{TG}} = -2$ V [Fig. S2(a)] to calculations for different values of $\theta$ [Fig. S2(b)–(e)]. For $\theta \leq 0.2°$, the $g_{\mathrm{Int}}$ vs. $V_{\mathrm{Int}}$ and $V_{\mathrm{BG}}$ characteristics do not change significantly. However, as highlighted by the dashed lines in Fig. S2(b)–(e), when $\theta$ increases beyond 0.2°, the primary resonance broadens and gets reduced in magnitude, as it is replaced by two resonances with an increasing separation in $V_{\mathrm{Int}}$ as the twist angle increases. From the comparison of measured data with calculations, we determine that the two graphene layer crystal axes are aligned within 0.2°.

To further illustrate the effect of an interlayer twist, Fig. S3(a) shows the measured $g_{\mathrm{Int}}$ vs. $V_{\mathrm{Int}}$ and $V_{\mathrm{TG}}$ at a fixed $V_{\mathrm{BG}} = 1$ V in a separate double monolayer graphene device using bilayer $WSe_2$ as tunnel barrier, and $\theta = 0.7°$. The data shows two tunneling resonances which evolve with $V_{\mathrm{Int}}$ and $V_{\mathrm{TG}}$. By identifying the location of the two interlayer biases $V_B$ at which the two layers Dirac cones begin to overlap, we can estimate $\theta = 0.7°$ in this additional device using $eV_B \approx 2\hbar v_F \Delta\mathbf{K}$ where $e$ is the electron charge. Furthermore, we find a good agreement between the measured data and calculation for the same value $\theta = 0.7°$ [Fig. S3(b)]. These datasets illustrate a method to assess if a relative twist exists between the layer crystal axes, and estimate its value.

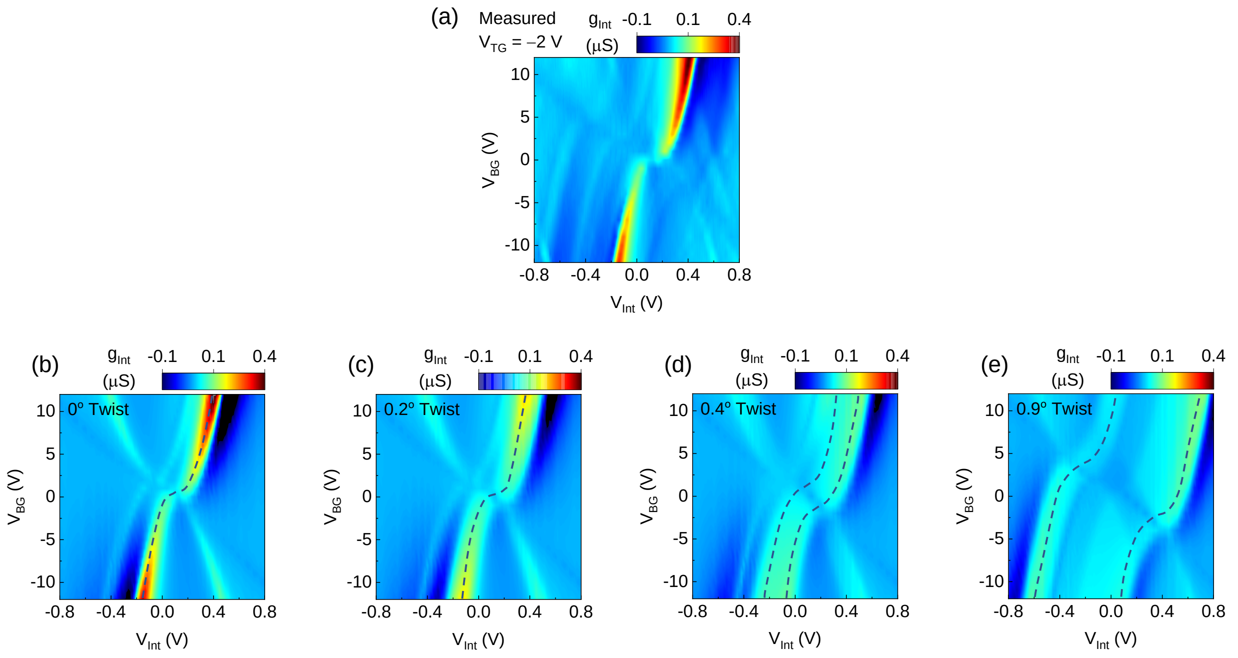


FIG. S2. (a) Measured $g_{\text{Int}}$ vs. $V_{\text{Int}}$ and $V_{\text{BG}}$ at a fixed $V_{\text{TG}} = -2$ V. (b)-(e) Calculated $g_{\text{Int}}$ for different values of $\theta$. The dashed lines indicate the single primary resonant tunneling conductance peak broadens and then splits into two as twist angle increases.

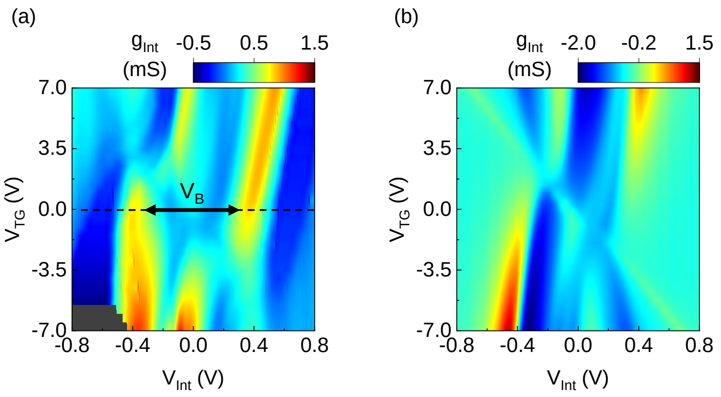


FIG. S3. (a) Measured $g_{\text{Int}}$ vs. $V_{\text{Int}}$ and $V_{\text{TG}}$ at a fixed $V_{\text{BG}} = 1$ V for an additional device with $\theta = 0.7°$. (b) Calculated $g_{\text{Int}}$ for the same biasing conditions as in panel (a), and $\theta = 0.7°$.

### III. Quantum oscillations in tunneling conductance at low magnetic fields

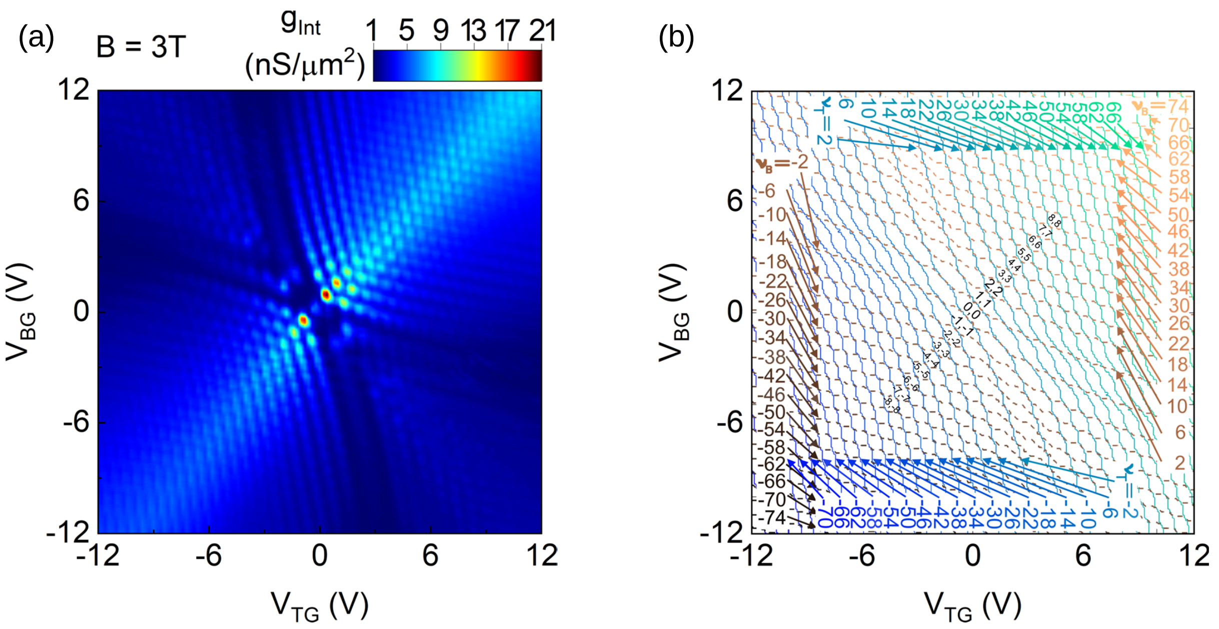


FIG. S4. (a) $g_{\mathrm{Int}}$ vs. $V_{\mathrm{TG}}$ and $V_{\mathrm{BG}}$ measured at $V_{\mathrm{Int}} = 0$ V, $B = 3$ T, and $T = 1.5$ K. (b) Calculated Landau level occupancy in each layer at $B = 3$ T. The integers mark the four-fold degenerate orbital Landau level indices.

## IV. Tunneling between uncorrelated landau levels

In Fig. S5, we use a single-particle tunneling model to rule out the scenario where extended states in individual, but otherwise uncorrelated layers lead to the observed zero-bias $g_{\rm Int}$ peak when the layers are at half-filling. The single particle tunneling between LLs of two graphene layers can be described using a model similar to that described in Eqs. (1)-(5) of the main text. We consider the tunneling process to strictly conserve the LL index $N$ and spin $\sigma$. However, we allow relaxation of valley degree of freedom $\sigma_v$ during tunneling. At high magnetic fields, the degeneracies in the LLs are lifted and the LL splitting is particularly prominent for $N = 0$ and $N = 1$ [4–6]. The tunneling rate in the presence of high magnetic fields is therefore given by

$$T(E) = \frac{A_{ov}}{h} \sum_{N;\sigma,\sigma_{vT},\sigma_{vB}} |t|^2 A_{\rm T}(N,\sigma,\sigma_{vT}) A_{\rm B}(N,\sigma,\sigma_{vB}). \tag{1}$$

Here, $A(N,\sigma,\sigma_v)$ is the Lorentizan-broadened spectral density function of the LL given by

$$A(N,\sigma,\sigma_v) = \frac{eB_\perp}{\pi h} \frac{\Gamma}{\left(E - \epsilon(N,\sigma,\sigma_v)\right)^2 + \Gamma^2}, \tag{2}$$

where $\epsilon(N,\sigma,\sigma_v)$ are the discretized LL energies, $B_\perp$ is the magnetic field applied entirely perpendicular to the sample and $A_{ov}$ is the overlap area between the top and bottom graphene layers.

The experimental zero-bias $g_{\rm Int}$ peaks shown in the insets of Fig. 3(a) and (b) are significantly sharper in high-magnetic fields compared to the $B = 0$ T data. Indeed, the single-particle model leads to a $g_{\rm Int}$ peak as a function of $V_{\rm Int}$ with a width similar to the experimental data of Fig. 3, only if using $\Gamma = 2$ meV, a value that is more than ten-fold smaller compared to the $\Gamma$ values of Figs. 1 and S3. Figure S5 shows the calculated $g_{\rm Int}$ vs. $V_{\rm Int}$ and $\Delta\nu_T = -\Delta\nu_B$ using this model for half-filled Landau levels. The single-particle model shows a $g_{\rm Int}$ peak that evolves with $V_{\rm Int}$, in clear contrast to experimental observations of Fig. 3(a-e) in the main text.

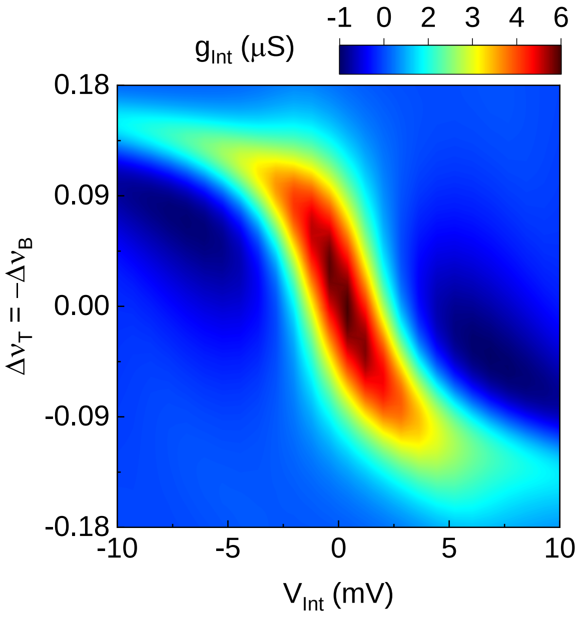


FIG. S5. Calculated $g_{\text{Int}}$ vs. $V_{\text{Int}}$ and $\Delta\nu_T = -\Delta\nu_B$ at $\nu = 3$ using a single-particle interlayer tunneling model, showing a $g_{\text{Int}}$ peak that evolves with $V_{\text{Int}}$, in contrast to experimental observations.

## V. Tunneling conductance dependence on magnetic field and temperature at $\nu = \pm 1, \pm 3$

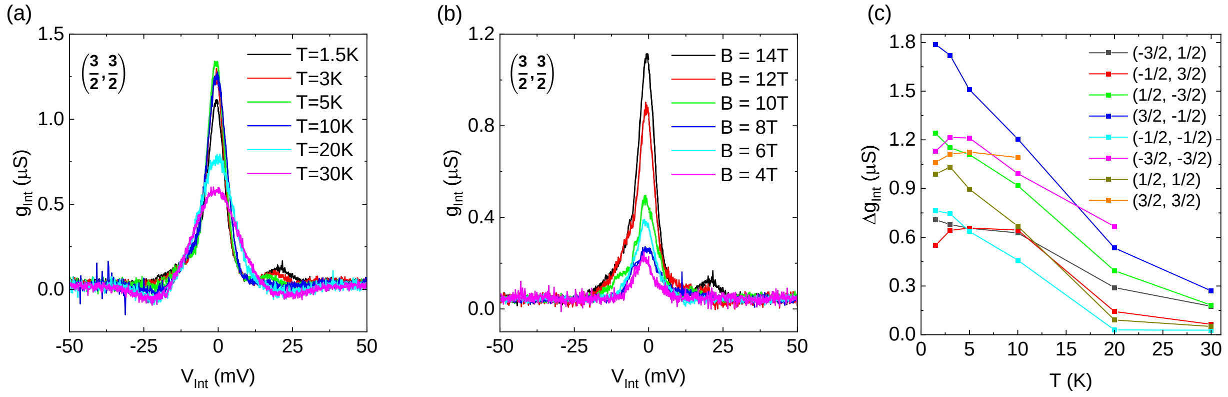


FIG. S6. (a) $g_{\mathrm{Int}}$ vs. $V_{\mathrm{Int}}$ at different $T$ values, at $B = 14$ T for $(\nu_{\mathrm{T}}, \nu_{\mathrm{B}}) = (3/2, 3/2)$. (b) $B$-dependence of $g_{\mathrm{Int}}$ vs. $V_{\mathrm{Int}}$ measured at $T = 1.5$ K for $(\nu_{\mathrm{T}}, \nu_{\mathrm{B}}) = (3/2, 3/2)$. (c) Interlayer conductance with the background tunneling removed ($\Delta g_{\mathrm{Int}}$) at $V_{\mathrm{Int}} = 0$ vs. $T$ measured at $B = 14$ T for various $\nu = \pm 1$ and $\pm 3$ states.

[1] A. Mishchenko, J. S. Tu, Y. Cao, R. V. Gorbachev, J. R. Wallbank, M. T. Greenaway, V. E. Morozov, S. V. Morozov, M. J. Zhu, S. L. Wong, et al., Nature Nanotech **9**, 808 (2014), URL https://doi.org/10.1038/nnano.2014.187.

[2] N. Prasad, G. W. Burg, K. Watanabe, T. Taniguchi, L. F. Register, and E. Tutuc, Phys. Rev. Lett. **127**, 117701 (2021), URL https://link.aps.org/doi/10.1103/PhysRevLett.127.117701.

[3] W.-Y. He, Y. Su, M. Yang, and L. He, Phys. Rev. B **89**, 125418 (2014), URL https://link.aps.org/doi/10.1103/PhysRevB.89.125418.

[4] Z. Jiang, Y. Zhang, H. L. Stormer, and P. Kim, Phys. Rev. Lett. **99**, 106802 (2007), URL https://link.aps.org/doi/10.1103/PhysRevLett.99.106802.

[5] A. F. Young, C. R. Dean, L. Wang, H. Ren, P. Cadden-Zimansky, K. Watanabe, T. Taniguchi, J. Hone, K. L. Shepard, and P. Kim, Nature Phys **8**, 550 (2012), URL https://doi.org/10.1038/nphys2307.

[6] S.-Y. Li, Y. Zhang, L.-J. Yin, and L. He, Phys. Rev. B **100**, 085437 (2019), URL https://link.aps.org/doi/10.1103/PhysRevB.100.085437.
